# Supplementary material for: A simple descriptor for energetics at fcc-bcc metal interfaces
Source: arXiv:1802.02957 ancillary file (2018-02-09)
Supplement: Supplementary file 1 [file suppinfo-Interface.pdf]

# Supporting information for: A simple descriptor for energetics at fcc-bcc metal interfaces

Linda A. Zotti,[*,†,‡] Stefano Sanvito,[‡] and David D. O'Regan[‡]

†*Departamento de Física Teórica de la Materia Condensada, Universidad Autónoma de Madrid, 28049 Madrid, Spain*

‡*School of Physics, AMBER and CRANN Institute, Trinity College Dublin, Dublin 2, Ireland*

E-mail: linda.zotti@uam.es

## Additional information on computed values of interface and surface energies

### Values in J/m$^2$

In Fig. S1 we show all values of interface and surface energies in J/m$^2$. The colour coded areas show the same trend as in Table 1 of the main text.

Table S1: Interface and surface energies in J/m$^2$

| | Cu | Ag | Au | Ni | Pd | Pt | Vacuum |
|---|---|---|---|---|---|---|---|
| Cr | 1.45 | 1.72 | 1.1941 | -0.091 | 0.094 | -0.223 | 3.93 |
| Mo | 0.99 | 1.52 | 0.8641 | -0.321 | -0.111 | -0.899 | 3.68 |
| W | 1.09 | 1.96 | 1.2613 | -0.487 | -0.04 | -0.646 | 4.49 |
| V | -0.18 | 0.36 | -0.532 | -1.099 | -1.217 | -1.589 | 2.8 |
| Nb | 0.17 | 0.78 | -0.717 | -1.009 | -1.532 | -1.844 | 2.72 |
| Ta | -0.3 | 0.7 | -0.647 | -1.706 | -1.617 | -1.935 | 2.88 |
| Vacuum | 2.07 | 1.31 | 1.44 | 2.97 | 2.22 | 2.4 | |

# Potential profile

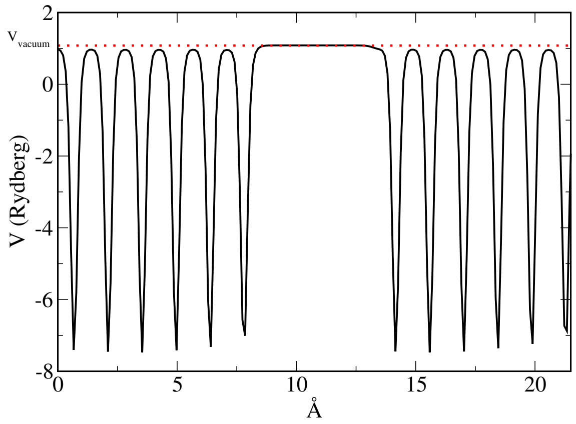


Figure S1: Example of the potential profile across a slab+vacuum system. Here, $V_{vacuum}$ indicates the vacuum potential used in Eq. 8 of the main text to calculate the work function.

## Experimental electronegativities

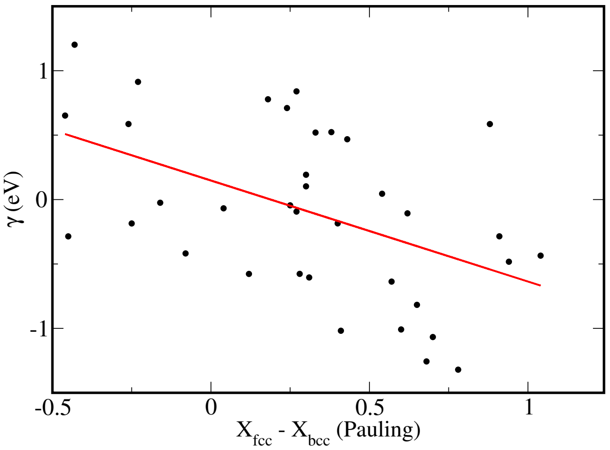


Figure S2: Interface energy as a function of the difference between the experimental electronegativities of the fcc and bcc metals. All values were obtained from https://www.webelements.com/

## Additional information on Löwdin charges

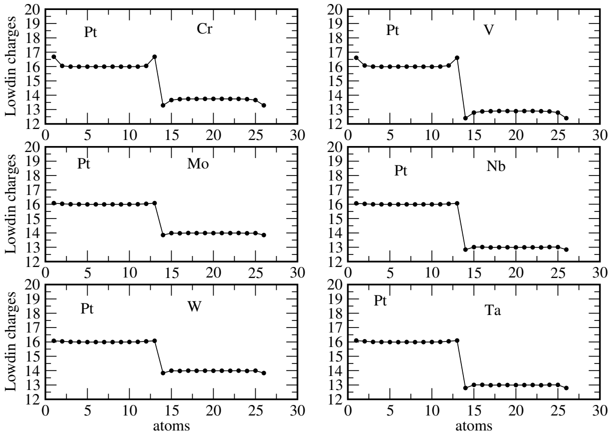


Figure S3: Pseudoatomic Löwdin charges for all Pt-bcc metal interfaces as an example: accumulation and depletion regions are formed at the interface due to the charge transfer taking place from each bcc metal to Pt.

# Geometric strain

| | Cu | Ag | Au |
|---|---|---|---|
| Cr | -0.307 | 0.0226 | 0.0564 |
| Mo | -0.583 | -0.285 | -0.254 |
| W | -0.606 | -0.316 | -0.284 |
| V | -0.432 | -0.09 | -0.071 |
| Nb | -0.661 | -0.453 | -0.422 |
| Ta | -0.659 | -0.447 | -0.422 |

| | Ni | Pd | Pt |
|---|---|---|---|
| Cr | -0.396 | -0.067 | -0.021 |
| Mo | -0.629 | -0.441 | -0.457 |
| W | -0.651 | -0.461 | -0.468 |
| V | -0.485 | -0.191 | -0.118 |
| Nb | -0.683 | -0.543 | -0.553 |
| Ta | -0.678 | -0.547 | -0.555 |

Figure S4: The strain experienced by each fcc metal lattice at the interface with each bcc metal (calculated as $a_{fcc}/\sqrt{2}$ in bulk phase - $a_{fcc}/\sqrt{2}$ in the interface).
